# Supplementary material for: Approximation capability of neural networks on spaces of probability measures and tree-structured domains
Source: arXiv:1906.00764 source file (2019-06-03)
Supplement: Supplementary file 1 [file appendix.tex]

%!TEX root = notes.tex
\begin{lemma}
Let $\mathcal{F}$ be a space of continuous functions defined on a compact set $\xspace.$ Then for all $a\in\asetf$ image of \pspace is a bounded subset of $\real.$ 
\end{lemma}

\begin{proof}[Proof of Lemma~\ref{lem:boundedimage}]
The proof starts by the fact that $a = \int f$
\end{proof}
